# Supplementary material for: Denoising Diffusion Probabilistic Models for Magnetic Resonance Fingerprinting
Source: arXiv:2410.23318 source file (2024-12-18)
Supplement: Supplementary file 1 [file supplementary.tex]

% \begin{center}
% \textbf{\large Supplemental Materials}
% \end{center}
\twocolumn[{%
 \centering
 \large \textbf{Supplementary Materials} \\[1.5em]
}]

%%%%%%%%%% Merge with supplemental materials %%%%%%%%%%
%%%%%%%%%% Prefix a "S" to all equations, figures, tables and reset the counter %%%%%%%%%%
\setcounter{equation}{0}
\setcounter{section}{0}
\setcounter{figure}{0}
\setcounter{table}{0}
\setcounter{page}{1}
\makeatletter

\renewcommand{\thefigure}{S\arabic{figure}}
\renewcommand \thesection{S\@arabic\c@section}
\renewcommand\thetable{S\@arabic\c@table}
\renewcommand \thefigure{S\@arabic\c@figure}
\makeatother
%%%%%%%%%% Prefix a "S" to all equations, figures, tables and reset the counter %%%%%%%%%%

% Figures to supplementary, table/plot in main manuscript
\begin{figure}
    \centering
    \setlength{\tabcolsep}{1pt}
      % \begin{tabularx}{\textwidth}{@{}*2{X}@{}}
      %   \includegraphics[width=\linewidth,trim={0.25cm 0.25cm 0.25cm 0.25cm},clip]{assets/t1_alternative_zoom.pdf}
      %   & \includegraphics[width=\linewidth,trim={0.25cm 0.25cm 0.25cm 0.25cm},clip]{assets/t2_alternative_zoom.pdf}
      % \end{tabularx}
    \includegraphics[width=\linewidth,trim={0.25cm 0.25cm 0.25cm 0.25cm},clip]{assets/t1_alternative_zoom.pdf}
\caption{Reconstructed T1 maps by our method and baselines along with percentage error maps for three representative brain slices from the evaluation set. Each slice is accompanied by two subfigures showcasing a zoomed-in version of a selected patch (top) and its corresponding error map (bottom). Electronic zooming is recommended.}
\label{fig:t1_maps_sup}
    
\end{figure}

\begin{figure}
    \centering
    \setlength{\tabcolsep}{1pt}
      % \begin{tabularx}{\textwidth}{@{}*2{X}@{}}
      %   \includegraphics[width=\linewidth,trim={0.25cm 0.25cm 0.25cm 0.25cm},clip]{assets/t1_alternative_zoom.pdf}
      %   & \includegraphics[width=\linewidth,trim={0.25cm 0.25cm 0.25cm 0.25cm},clip]{assets/t2_alternative_zoom.pdf}
      % \end{tabularx}
    \includegraphics[width=\linewidth,trim={0.25cm 0.25cm 0.25cm 0.25cm},clip]{assets/t2_alternative_zoom.pdf}
\caption{Reconstructed T2 maps by our method and baselines along with percentage error maps for three representative brain slices from the evaluation set. Each slice is accompanied by two subfigures showcasing a zoomed-in version of a selected patch (top) and its corresponding error map (bottom). Electronic zooming is recommended.}
\label{fig:t2_maps_sup}
    
\end{figure}
